# Supplementary material for: Myocardial Architecture and Patient Variability in Clinical Patterns of Atrial Fibrillation
Source: arXiv:1606.03910 source file (2016-06-13)
Supplement: Supplementary file 1 [file SupplementaryInformation.pdf]

## Supplementary Information

### The Model

We provide a brief summary of the model and parameters used. The tissue is represented by a $L \times L$ square grid of discrete cells. Heart muscle tissue forms a branching network of interacting cells where each cell is coupled to its neighbors longitudinally and to its neighbors transversally with probability $\nu$. The structure of the lattice can be considered to be a set of aligned longitudinal cables of single cell thickness which are coupled to neighboring cables with frequency $\nu$. The lateral uncoupling of cells is thus represented by reducing the frequency of vertical couplings through the parameter $\nu$. To represent the simplest features of an atrium we apply periodic boundary conditions vertically and open boundary conditions horizontally to the 2D model giving a cylindrical topology which is a convenient substrate to study the evolution of wave fronts. Cells along the left boundary are pacemakers and self-excite at a fixed period $T^{'} = 660ms$ to mimic normal cardiac rhythm.

Simplifying the action potential, a cell may be in one of three states: resting (repolarized), excited (depolarizing), or refractory. An excited cell causes neighboring coupled resting cells to become excited. Thus the wave front is a coherent propagation of this excitation throughout the tissue.A healthy atrial area is $L^{'} \times L^{'} \approx 20cm^2$. Atrial muscle tissue is made of nearly cylindrical myocytes of length $\Delta x' \approx 100\mu$m and diameter $\Delta y' \approx 20\mu$m packed in an irregular brick-wall like pattern. The time taken for a cell to depolarize,$\Delta t' \approx 0.6$ms, is much shorter than the refractory period, $\tau' \approx 150$ms.

Cellular electrical dysfunction of any cause can introduce a degree of noise into the excitation process. A fraction  of randomly chosen cells in the lattice are chosen to be dysfunctional. Such cells have a finite probability  of not exciting in response to an excited neighbor and hence can block the propagation of activation.

Translating real tissue values into the model gives$L = L^{'}/\Delta x' = 1000$. We coarse grain the model by taking $\Delta x' \rightarrow b\Delta x'$, where $b$ is the number of cells within a unit of space in the model. As the conduction velocity $\theta'_x = \Delta x'/\Delta t' \approx 0.2\text{ms}^{-1}$ is fixed we also find $\Delta t' \rightarrow b\Delta t'$. We take $b = 5$ implying that the parameters of the model are system size $L = 200$, refractory period $\tau = \tau'/(b\Delta t') = 50$, the fraction of dysfunctional cells $\delta = 0.05$, the

probability of dysfunction $\epsilon = 0.05$, the period of pacing $T = T'/(b\Delta t') = 220$ using $T' = 660$ms, leaving the fraction of transverse connections as the only control parameter. See our previous paper10 for a detailed discussion on the model.

## Full dataset of all 32 simulations

We present the results of all 32 simulated "patients". We start at $\nu = 0.25$ where all the simulated heart muscle tissue are in sinus rhythm (SR) but as we lower $\nu$, fibrillation emerges. The initial conditions for each "patient" are created by assigning the same number of vertical connections (identical initial $\nu$) but at different random positions. Next the accumulation of cellular uncoupling is implemented by reducing $\nu$ (e.g., to mimic the progression of fibrosis or gap junctional uncoupling). To do this, we run simulations for a period of $T = 4.3 \times 10^7$ time steps in the computer model and vertical connections are removed at a rate of one connection every nine thousand time steps. We observe the dynamics of excitation wavefronts as the transversal uncoupling accumulates in the tissue. All other model parameters are set to physiological values: $L = 200$, $\tau = 50$, $\epsilon = 0.05$, and $\delta = 0.05$. Pacemaker cells self-activate with a period of $T = 220$.

The AF burden and number of critical regions versus fraction of vertical connections is shown in supplementary Fig. 1 to 4. We show the average AF burden as a function of the number of critical regions for each simulation in supplementary Fig. 5.

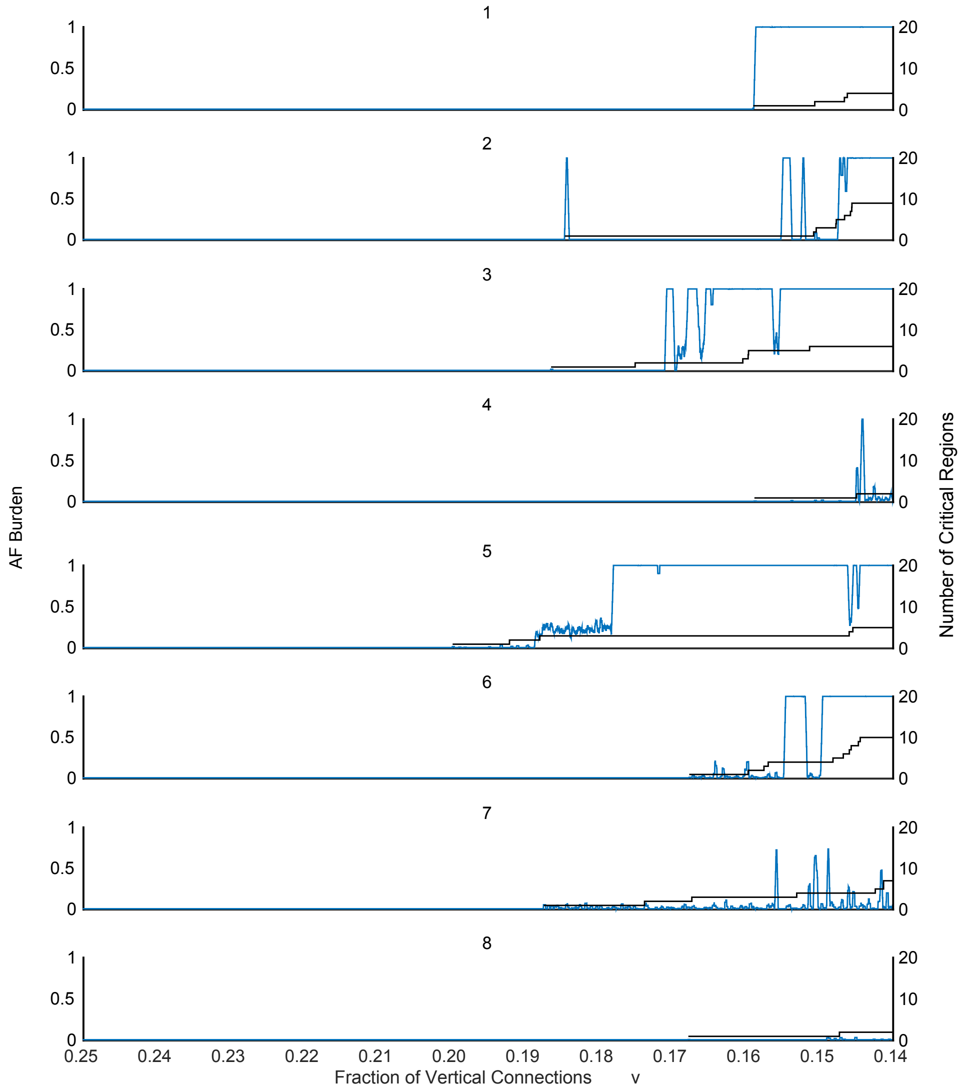


**Supplementary Figure 1:** AF burden (blue) varies with time, calculated from the time in AF in a sliding window of $5 \times 10^6$ time steps for simulations 1 to 8. Also shown is the accumulation of initiating critical regions (black curve) versus the fraction of vertical connections

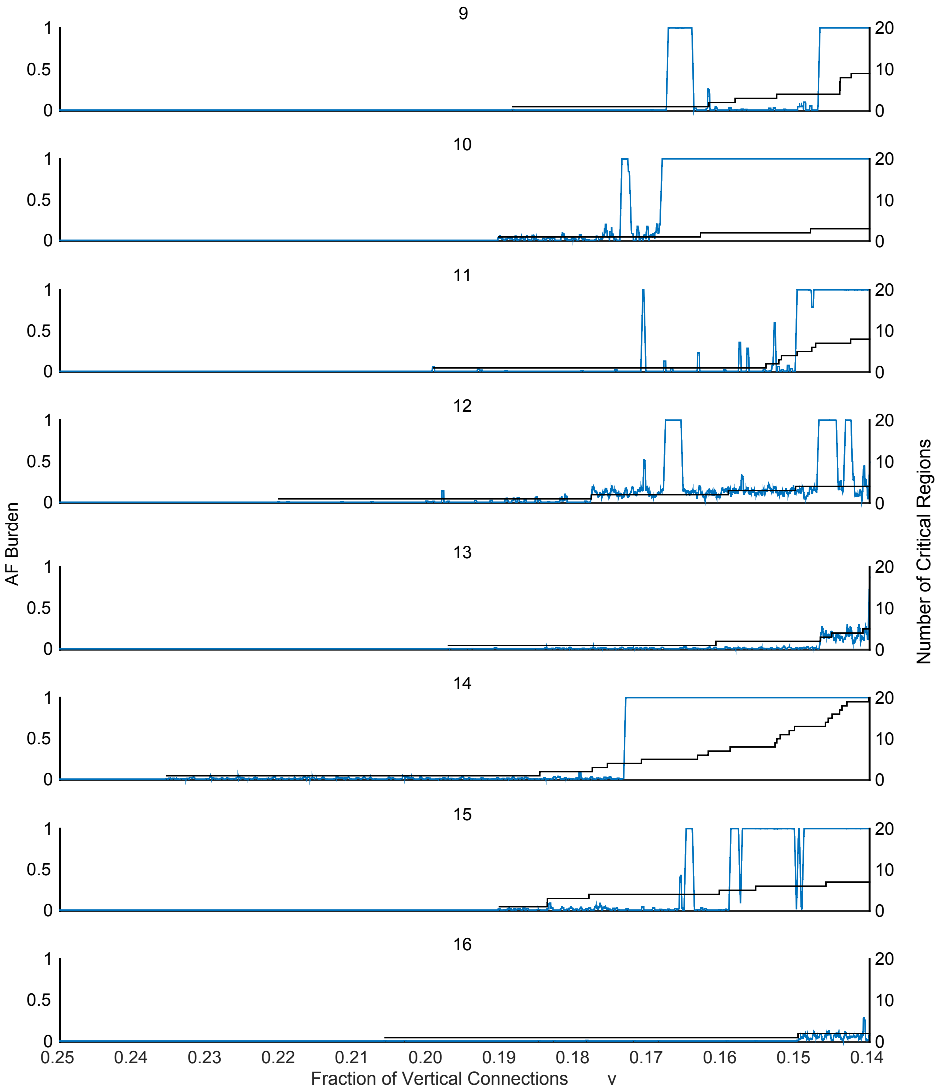


**Supplementary Figure 2:** AF burden (blue) varies with time, calculated from the time in AF in a sliding window of $5 \times 10^6$ time steps for simulations 9 to 16. Also shown is the accumulation of initiating critical regions (black curve) versus the fraction of vertical connections

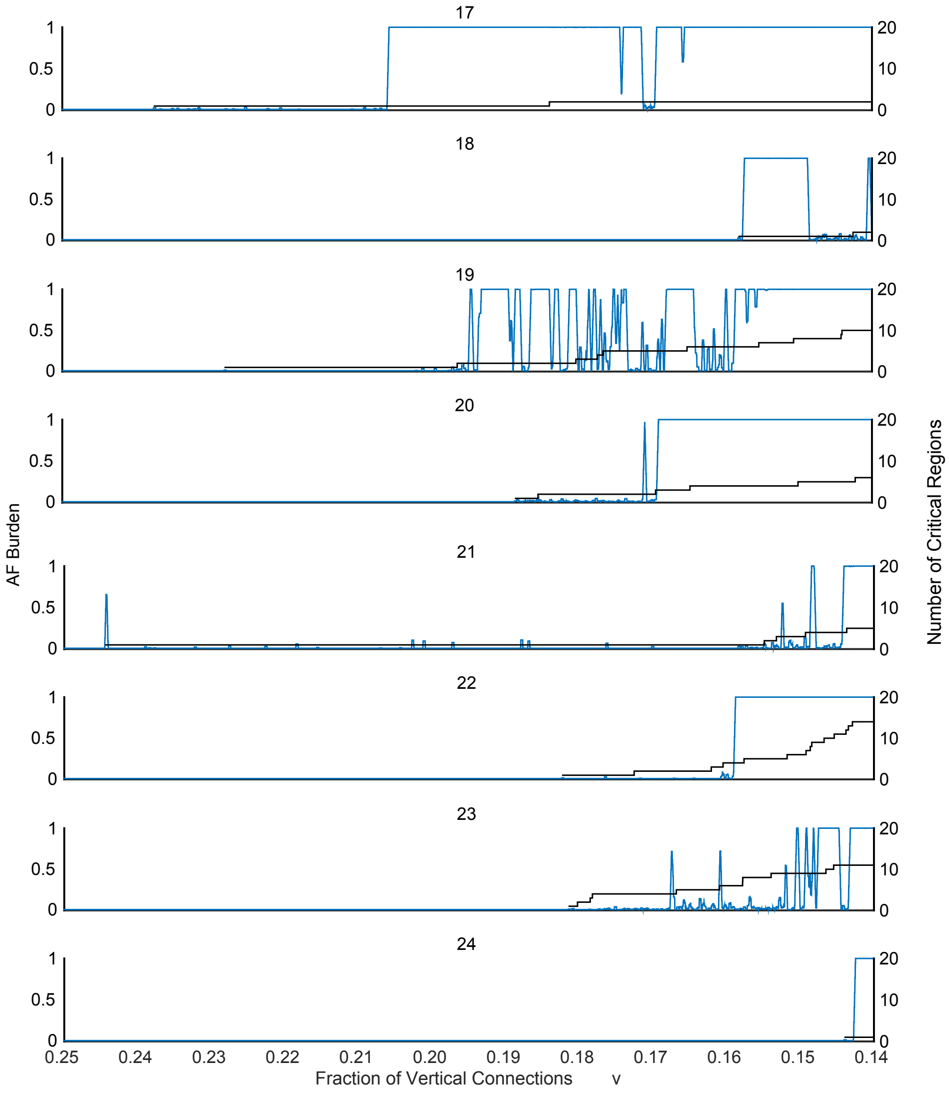


**Supplementary Figure 3:** AF burden (blue) varies with time, calculated from the time in AF in a sliding window of $5 \times 10^6$ time steps for simulations 17 to 24. Also shown is the accumulation of initiating critical regions (black curve) versus the fraction of vertical connections

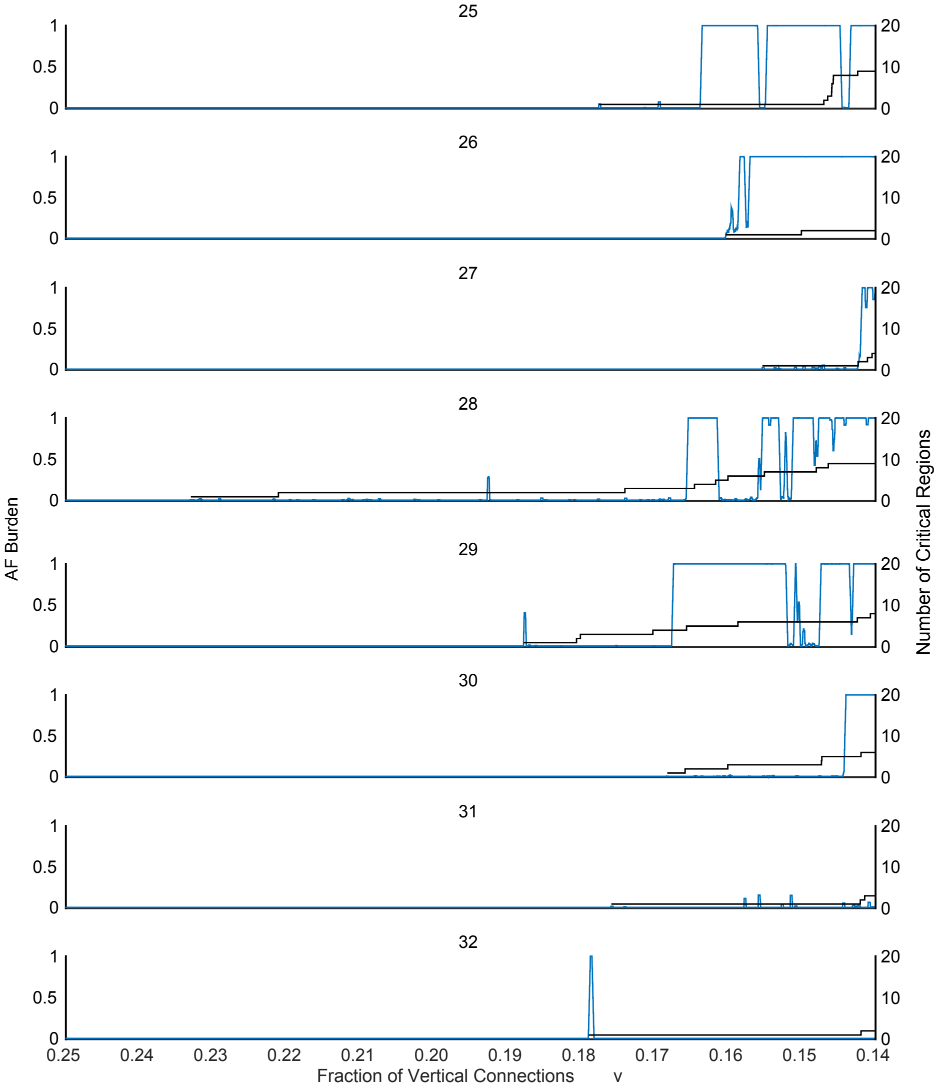


**Supplementary Figure 4:** AF burden (blue) varies with time, calculated from the time in AF in a sliding window of $5 \times 10^6$ time steps for simulations 25 to 32. Also shown is the accumulation of initiating critical regions (black curve) versus the fraction of vertical connections

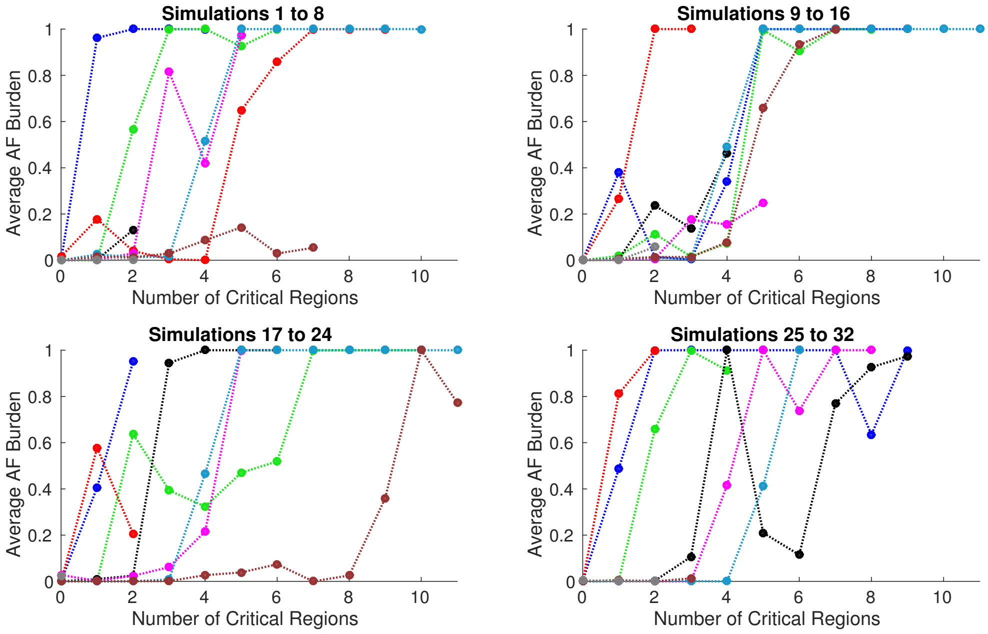


**Supplementary Figure 5:** The average AF burden for all 32 simulations as a function of the number of critical regions. The standard deviations and standard error are too small to be seen at this scale. The differences in the accumulation of critical regions between patients better predicts the variability in the AF behaviour observed.
